# Supplementary material for: p-State Luminescence in CdSe Nanoplatelets: The Role of Lateral Confinement and an LO Phonon Bottleneck
Source: arXiv:1507.05465 ancillary file (2015-07-20)
Supplement: Supplementary file 1 [file Platelets_SuppInf.pdf]

# Supporting Information: p-State Luminescence in CdSe Nanoplatelets: The Role of Lateral Confinement and an LO-Phonon Bottleneck

Alexander W. Achtstein†,[1,*] Riccardo Scott,[1,†] Sebastian Kickhöfel,[1] Stefan T. Jagsch,[2] Sotirios Christodoulou,[3,4] Anatol V. Prudnikau,[5] Artsiom Antanovich,[5] Mikhail Artemyev,[5] Iwan Moreels,[4] Andrei Schliwa,[2] and Ulrike Woggon[1]

[1]*Institute of Optics and Atomic Physics, Technical University of Berlin, Strasse des 17. Juni 135, 10623 Berlin, Germany*

[2]*Institute of Solid State Physics, Technical University of Berlin, Strasse des 17. Juni 135, 10623 Berlin, Germany*

[3]*Department of Physics, University of Genoa, via Dodecaneso 33, IT-16146 Genova, Italy*

[4]*Istituto Italiano di Tecnologia, Via Morego 30, IT-16163 Genova, Italy*

[5]*Institute for Physico-Chemical Problems, Belarusian State University, 220030 Minsk, Belarus*

[*] alexander.achtstein@tu-berlin.de; Current address: Optoelectronic Materials Section, Delft University of Technology, 2628 BL Delft, The Netherlands

[†] R.S. and A.W.A. contributed equally to this work.

**Synthesis and Characterization:**

CdSe core NPls with the first exciton absorption bands around 512 nm (4.5 ML) and 17x6, 29x8, 30x15 and 41x13 $nm^2$ lateral size were synthesized as described in Ref. 1. Absorption and PL spectra as well as TEM images are shown in Fig. 1. Core CdSe NPLs with 21x7 $nm^2$ lateral extensions were synthesized as in Ref. 2. In line with results of She et al.[3] we assume our NPLs to be Cd terminated on both basal planes. The results of a TEM size analysis are shown in Table I. The particles were redissolved in toluene and embedded in PMAO polymer (from Aldrich) on thin fused silica substrates and mounted in a Cryovac Conti IT

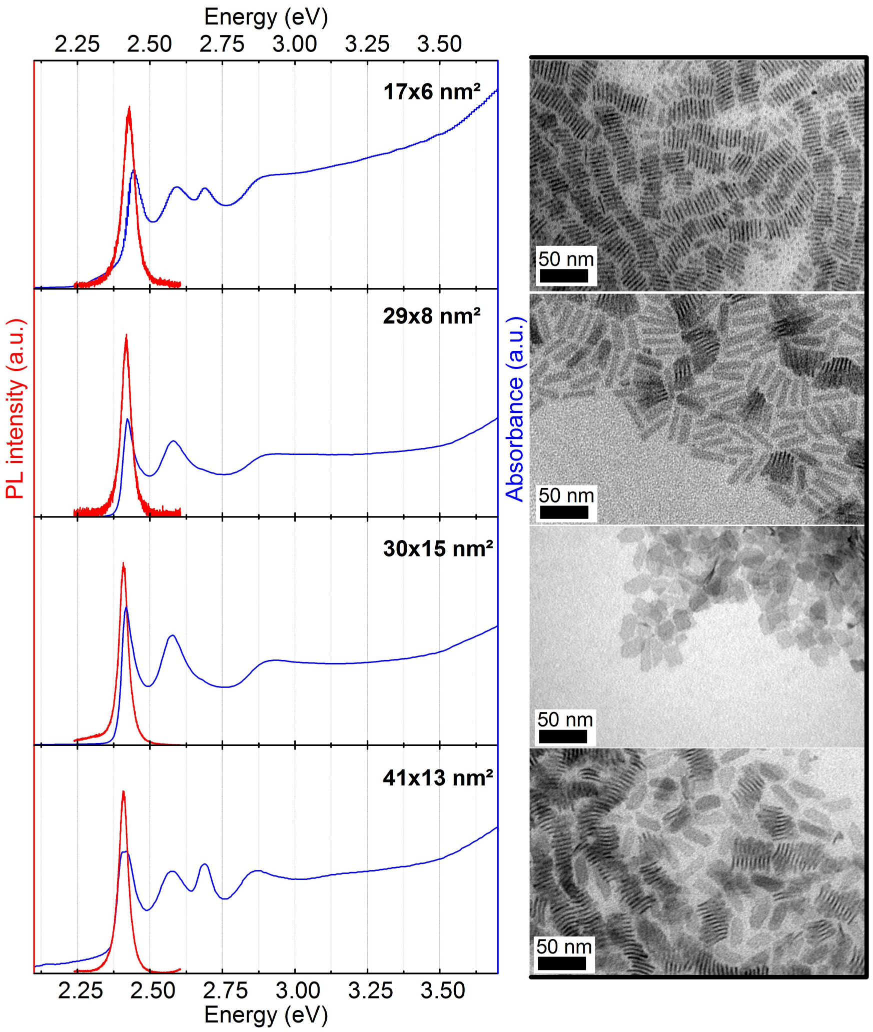


FIG. 1. Room temperature photoluminescence (red) and absorption (blue) spectra and corresponding TEM images of 4.5 ML CdSe core NPLs. The average lateral sizes are noted for each NPL population.

cryostat (3.5-300 K). The volume fraction in the polymer was kept below 1 % to avoid any aggregation or FRET effects [4].

CdSe-Cds core-wing NPLs were synthesized as described in Ref. 5. A PL spectrum of these CdSe-CdS core-wing NPLs at 4 K with fits to determine the ES-GS energy spacing is shown in Fig. 2.

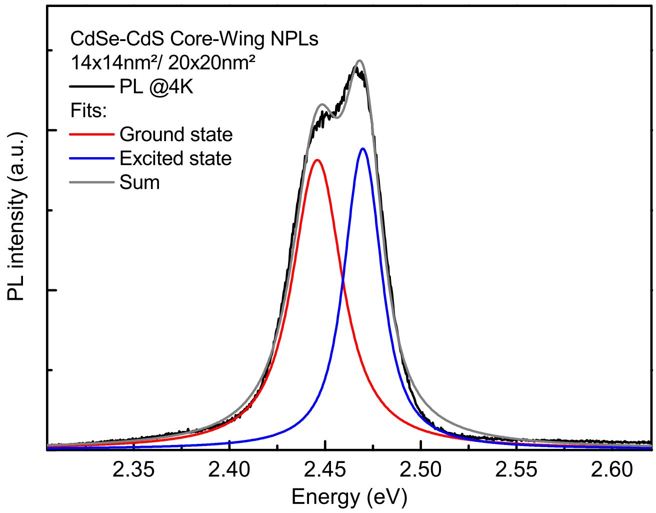


FIG. 2. 4 K PL spectra of CdSe-CdS core-lateral shell NPLs with 14x14 $nm^2$ CdSe core and 20x20 $nm^2$ CdS lateral shell. The red and blue curves result from Voigt-profile fits to derive the peak positions of ground state (red) and excited state emission (blue).

**Experimental Setup:**

Our experimental setup allows the consecutive measurement of time-integrated and -resolved fluorescence of a sample with confocal excitation (SHG of a titanium sapphire laser at 420 nm (Coherent Mira 900F, FWHM 150 fs, 75,4 MHz)) and detection (N.A.=0.4) through an objective. A spectrometer with an attached CCD (Roper Spec10) for time-integrated or a streak camera (Hamamatsu C5680) for time-resolved measurements are used. The excitation density was held below moderate 0.2 $W/cm^2$ to avoid any heating and saturation effects (we estimate only $< 0.1$ percent of the platelets are excited within one laser pulse using ICP and absorption cross sections of She et al. [3]). These low densities also rule out the presence of biexcitons.

**Theory and Results Table:**

As in our previous work [6] the electronic structure on the nanoplatlets is obtained using a 3D implementation of eight-band $\mathbf{k}\cdot\mathbf{p}$ envelope function theory. Following the discussion in [7] we implemented the self-energy term for the Coulomb term in our Hartree approach. Both, the effects arising from the dielectric environment and the electron and hole self-energy are included. We employed the following dielectric constants: $\epsilon_r^{Platelet} = 9.4$ and $\epsilon_r^{out} = 4.0$. The following table I summarizes the experimental and theoretical GS energies $E_{GS}$ and the corresponding ES-GS energy spacings $\Delta E$.

TABLE I. Sizes, hh ground state emission $E_{GS}$ at 4 K, and energy difference between ground state and excited state emission $\Delta E$ of the investigated CdSe core NPLs extracted from PL measurements (PL) and calculated values (Theo).

| Size ($nm^2$) | $E_{GS}^{(PL)}$ (eV) | $\Delta E^{(PL)}$ (meV) | $E_{GS}^{(Theo)}$ (eV) | $\Delta E^{(Theo)}$ (meV) |
|---|---|---|---|---|
| 17x6 | 2.486 | 36 | 2.485 | 41 |
| 21x7 | 2.480 | 32 | 2.477 | 35 |
| 29x8 | 2.469 | 27 | 2.465 | 27 |
| 30x15 | 2.466 | 20 | 2.447 | 22 |
| 41x13 | 2.488 | 18 | 2.449 | 22 |
| 14x14[a] | 2.446 | 24 | 2.471 | 28 |

[a] Core size of CdSe/CdS core (14x14 $nm^2$) lateral shell (20x20 $nm^2$) NPLs.

[1] J. Q. Grim, S. Christodoulou, F. Di Stasio, R. Krahne, R. Cingolani, L. Manna, and I. Moreels, Nature Nanotechnology **9**, 891 (2014).

[2] A. W. Achtstein, A. V. Prudnikau, M. V. Ermolenko, L. I. Gurinovich, S. V. Gaponenko, U. Woggon, A. V. Baranov, M. Y. Leonov, I. D. Rukhlenko, A. V. Fedorov, and M. V. Artemyev, ACS Nano **8**, 7678 (2014).

[3] C. She, I. Fedin, D. S. Dolzhnikov, A. Demortière, R. D. Schaller, M. Pelton, and D. V. Talapin, Nano Lett. **14**, 2772 (2014).

[4] B. Guzelturk, O. Erdem, M. Olutas, Y. Kelestemur, and H. V. Demir, ACS Nano , 12524 (2014).

[5] A. Prudnikau, A. Chuvilin, and M. Artemyev, J. Am. Chem. Soc. **135**, 14476 (2013).

[6] A. W. Achtstein, A. Schliwa, A. Prudnikau, M. Hardzei, M. V. Artemyev, C. Thomsen, and U. Woggon, Nano Lett. **12**, 3151 (2012).

[7] R. Benchamekh, N. A. Gippius, J. Even, M. O. Nestoklon, J.-M. Jancu, S. Ithurria, B. Dubertret, A. L. Efros, and P. Voisin, Phys. Rev. B **89**, 035307 (2014).
